# Supplementary material for: A single-cell mathematical model of SARS-CoV-2 induced pyroptosis and the effects of anti-inflammatory intervention
Source: arXiv:2008.04172 source file (2021-03-29)
Supplement: Supplementary file 1 [file Supplementary_Material.pdf]

# Supplementary Material

for ‘A single-cell mathematical model of SARS-CoV-2 induced pyroptosis and the effects of anti-inflammatory intervention’ by S J Hamis and F R Macfarlane

## Contents

|                                                           |    |
|-----------------------------------------------------------|----|
| S1 Modifying the modelled nuclear NF- $\kappa$ B peak     | 1  |
| S2 Results from the robustness sensitivity analysis       | 1  |
| S3 Results from the global sensitivity analysis           | 23 |
| S4 Results from the derivative-based sensitivity analysis | 23 |

## S1 Modifying the modelled nuclear NF- $\kappa$ B peak

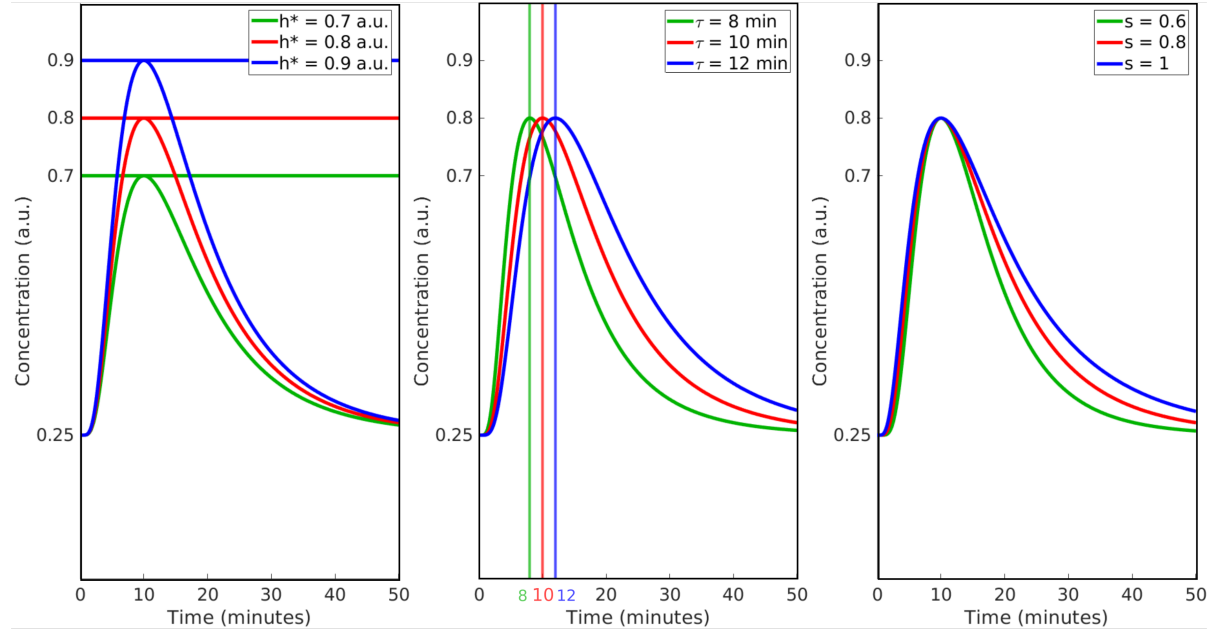

Figure S1.A: The parameters  $h^* = [\text{NF-}\kappa\text{B}_n](0) + h$ ,  $\tau$ , and  $s$  can be adjusted to modify the shape of the phenomenologically modelled  $[\text{NF-}\kappa\text{B}_n]$  peak. In the figure,  $h^*$ ,  $\tau$  and  $s$  are varied one at a time from the baseline values ( $[\text{NF-}\kappa\text{B}_n](0) = 0.25$  a.u.,  $h = 0.55$  a.u.,  $\tau = 10$  min,  $s = 0.8$ ). Here,  $[\text{NF-}\kappa\text{B}_n](0)$  denotes the nuclear NF- $\kappa$ B levels prior to pyroptosis-initiating signalling,  $h$  denotes the peak-value elevation of nuclear NF- $\kappa$ B,  $\tau$  denotes the time that the nuclear NF- $\kappa$ B levels peak, and  $s$  denotes the skewness of the peak.

## S2 Results from the robustness sensitivity analysis

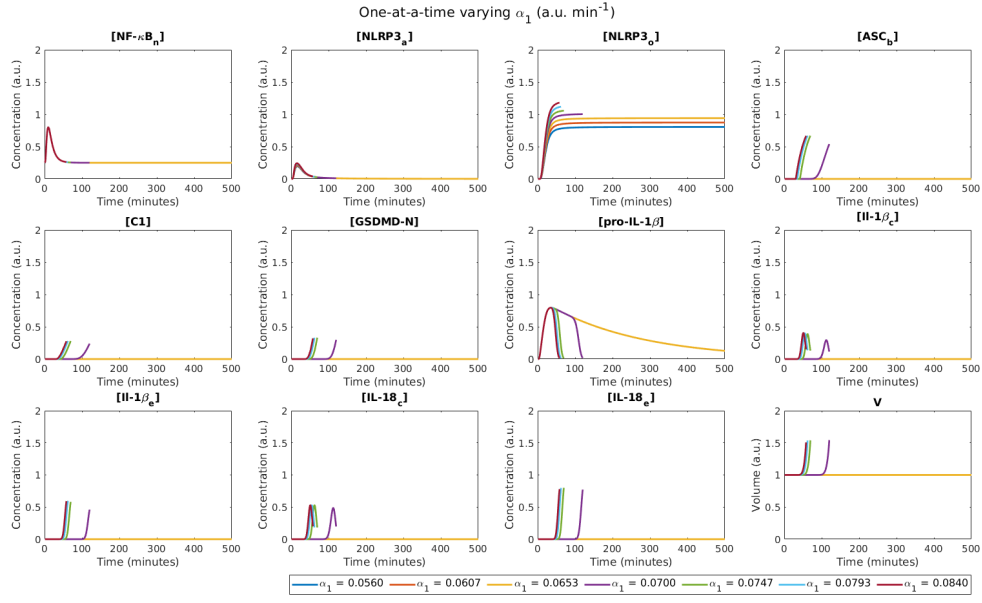

Figure S2.B: Numerical simulations results of the ODE model, while testing a range of values of the parameter  $\alpha_1$  and fixing all other parameter values. We display the concentration of each model component in arbitrary units (a.u.) over time, as well as cell volume dynamics for each of the values tested. Note that the time progression stops once the critical volume  $V_c = 1.5$  is reached and the ultimate cell membrane rupture occurs.

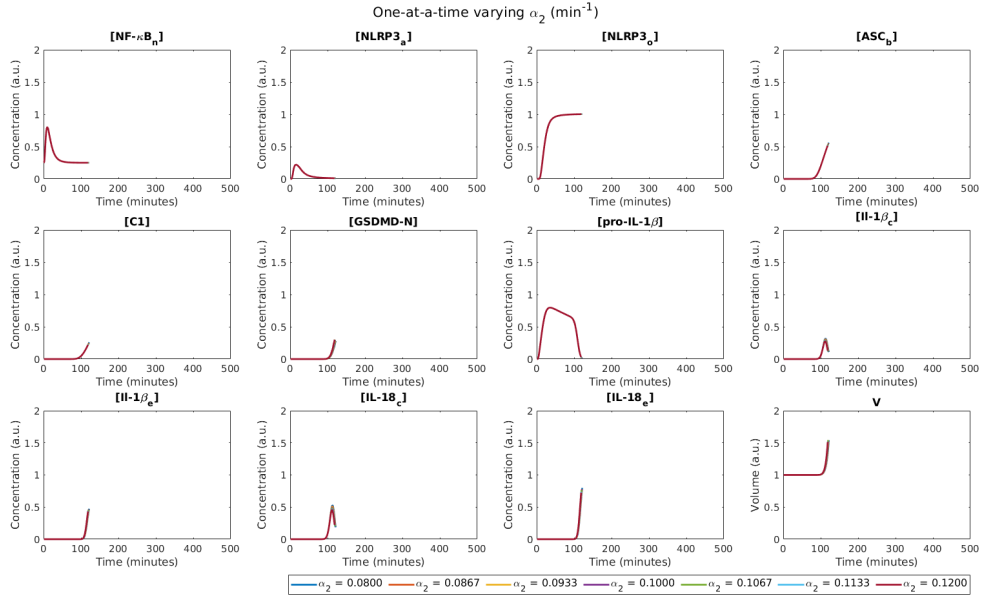

Figure S2.C: Numerical simulations results of the ODE model, while testing a range of values of the parameter  $\alpha_2$  and fixing all other parameter values. We display the concentration of each model component in arbitrary units (a.u.) over time, as well as cell volume dynamics for each of the values tested. Note that the time progression stops once the critical volume  $V_c = 1.5$  is reached and the ultimate cell membrane rupture occurs.

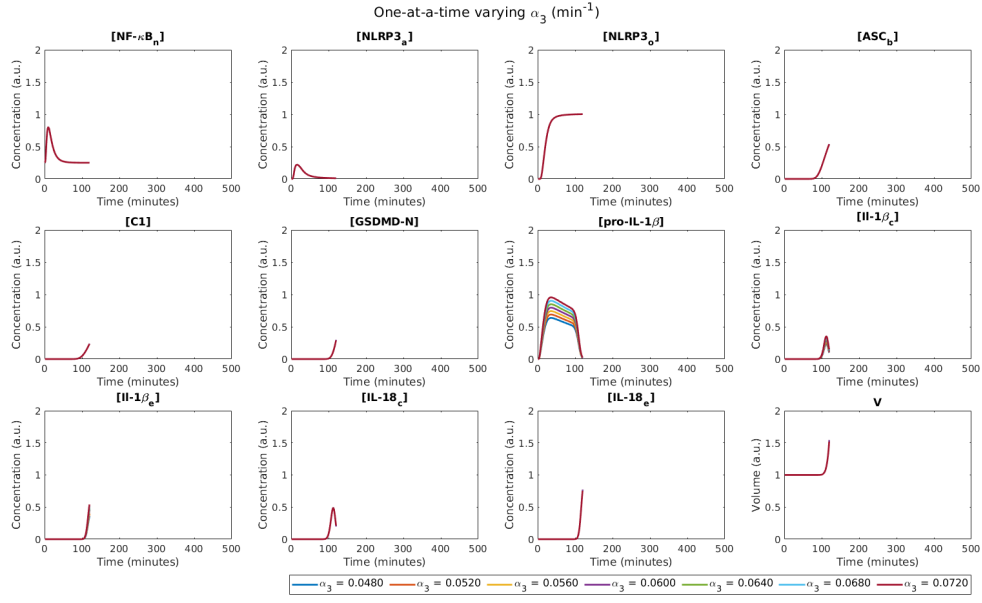

Figure S2.D: Numerical simulations results of the ODE model, while testing a range of values of the parameter  $\alpha_3$  and fixing all other parameter values. We display the concentration of each model component in arbitrary units (a.u.) over time, as well as cell volume dynamics for each of the values tested. Note that the time progression stops once the critical volume  $V_c = 1.5$  is reached and the ultimate cell membrane rupture occurs.

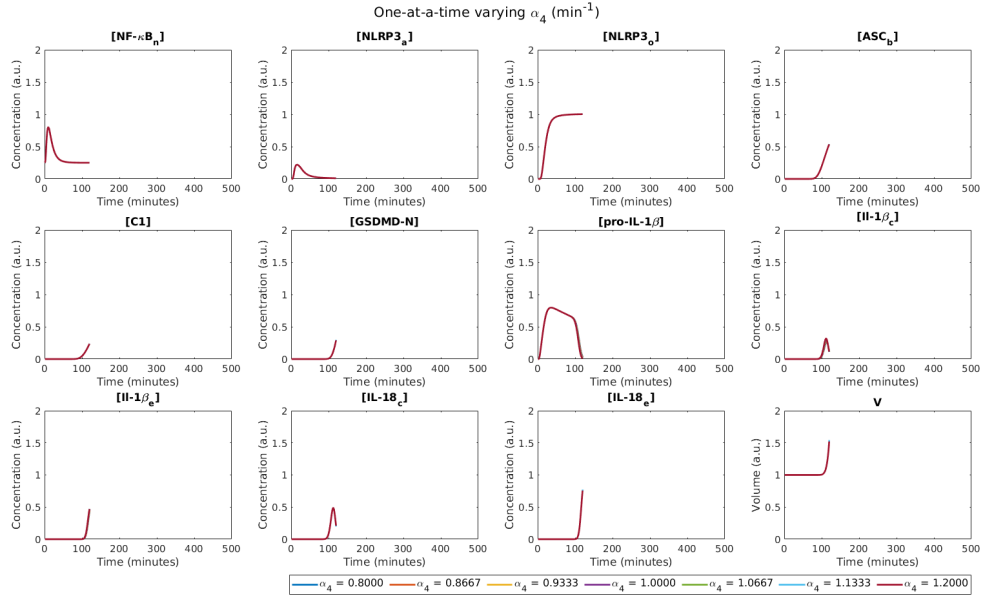

Figure S2.E: Numerical simulations results of the ODE model, while testing a range of values of the parameter  $\alpha_4$  and fixing all other parameter values. We display the concentration of each model component in arbitrary units (a.u.) over time, as well as cell volume dynamics for each of the values tested. Note that the time progression stops once the critical volume  $V_c = 1.5$  is reached and the ultimate cell membrane rupture occurs.

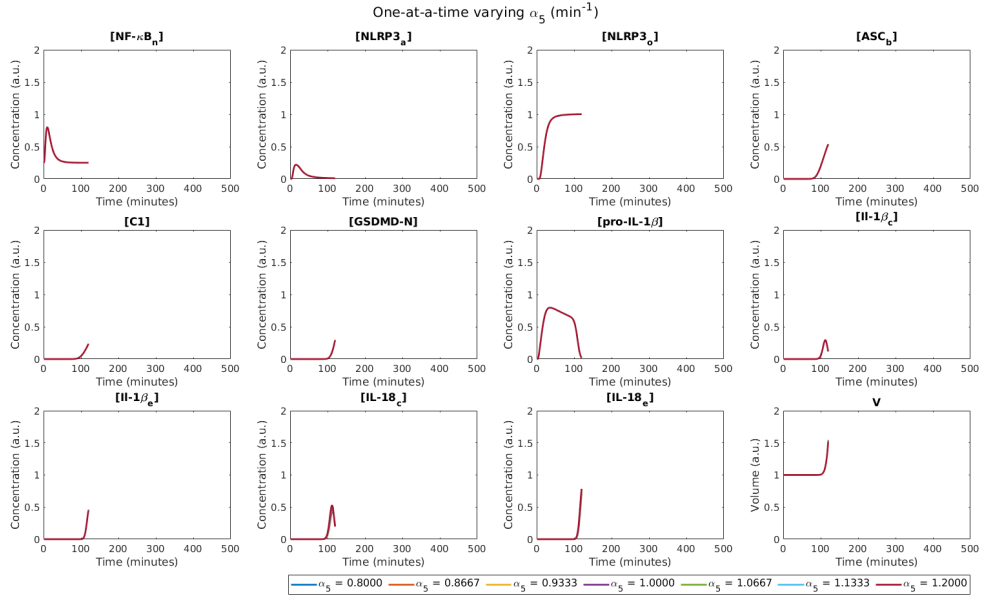

Figure S2.F: Numerical simulations results of the ODE model, while testing a range of values of the parameter  $\alpha_5$  and fixing all other parameter values. We display the concentration of each model component in arbitrary units (a.u.) over time, as well as cell volume dynamics for each of the values tested. Note that the time progression stops once the critical volume  $V_c = 1.5$  is reached and the ultimate cell membrane rupture occurs.

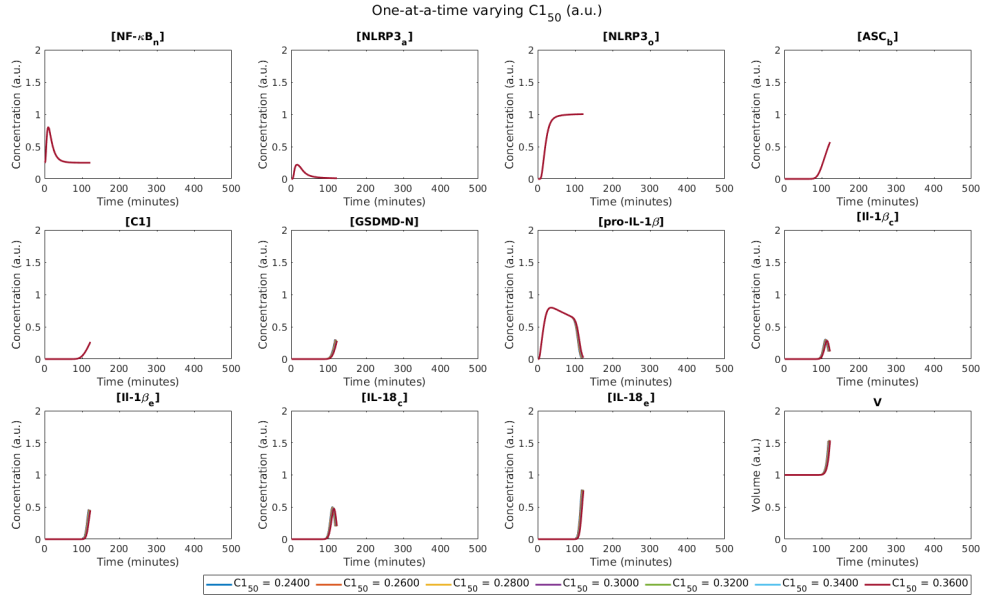

Figure S2.G: Numerical simulations results of the ODE model, while testing a range of values of the parameter  $C1_{50}$  and fixing all other parameter values. We display the concentration of each model component in arbitrary units (a.u.) over time, as well as cell volume dynamics for each of the values tested. Note that the time progression stops once the critical volume  $V_c = 1.5$  is reached and the ultimate cell membrane rupture occurs.

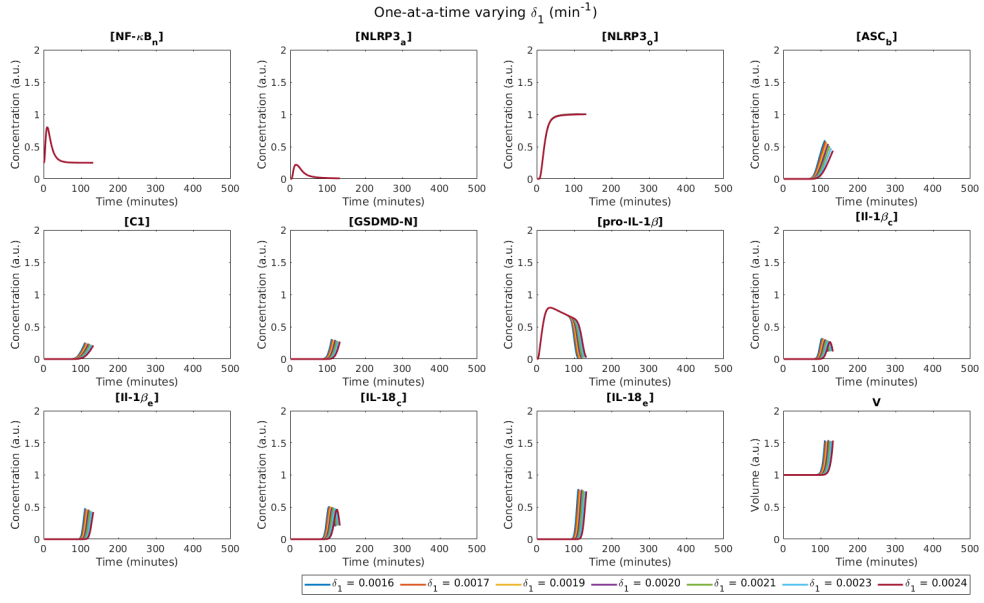

Figure S2.H: Numerical simulations results of the ODE model, while testing a range of values of the parameter  $\delta_1$  and fixing all other parameter values. We display the concentration of each model component in arbitrary units (a.u.) over time, as well as cell volume dynamics for each of the values tested. Note that the time progression stops once the critical volume  $V_c = 1.5$  is reached and the ultimate cell membrane rupture occurs.



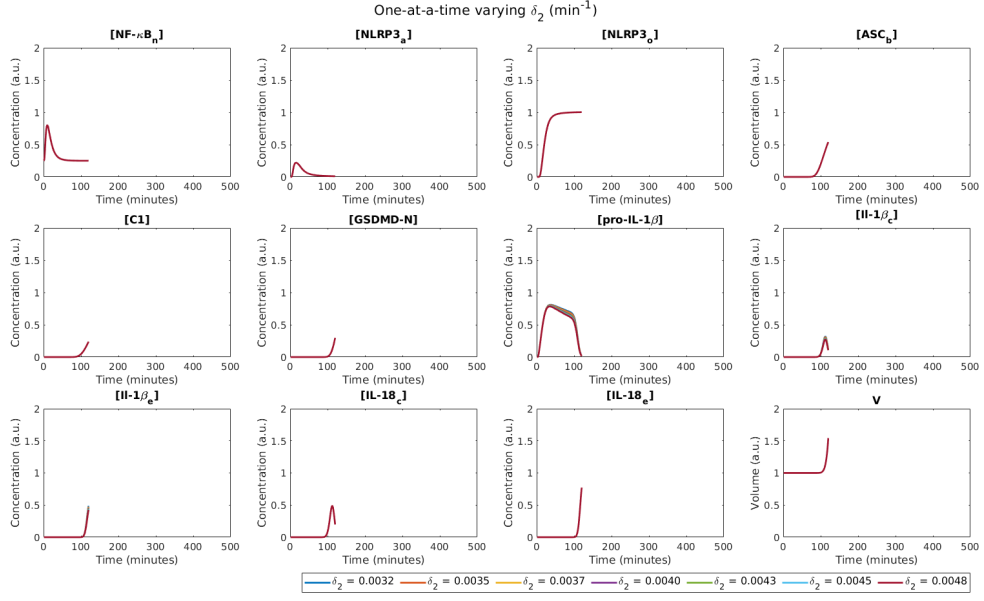

Figure S2.I: Numerical simulations results of the ODE model, while testing a range of values of the parameter  $\delta_2$  and fixing all other parameter values. We display the concentration of each model component in arbitrary units (a.u.) over time, as well as cell volume dynamics for each of the values tested. Note that the time progression stops once the critical volume  $V_c = 1.5$  is reached and the ultimate cell membrane rupture occurs.

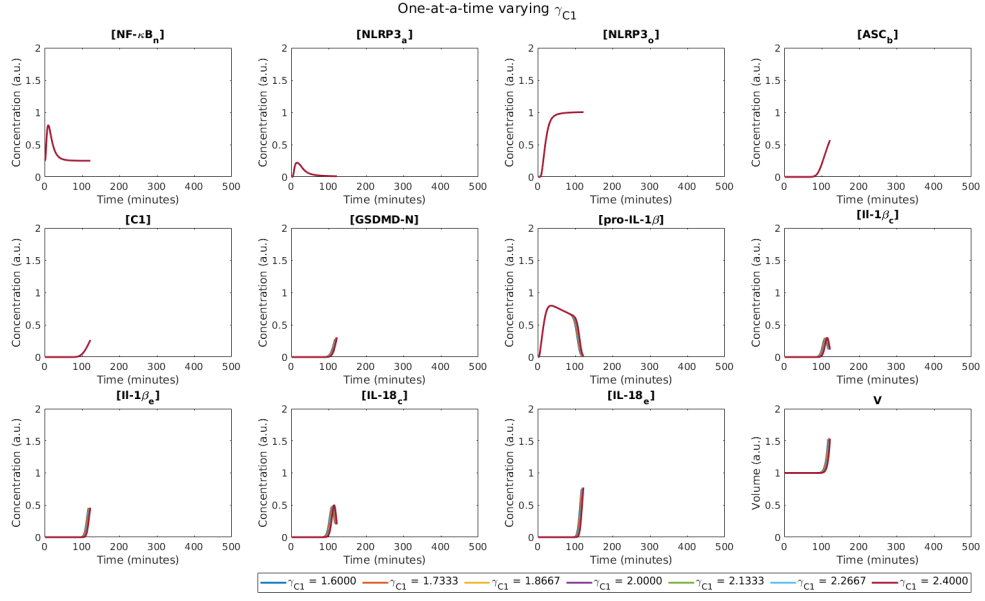

Figure S2.J: Numerical simulations results of the ODE model, while testing a range of values of the parameter  $\gamma_{C1}$  and fixing all other parameter values. We display the concentration of each model component in arbitrary units (a.u.) over time, as well as cell volume dynamics for each of the values tested. Note that the time progression stops once the critical volume  $V_c = 1.5$  is reached and the ultimate cell membrane rupture occurs.

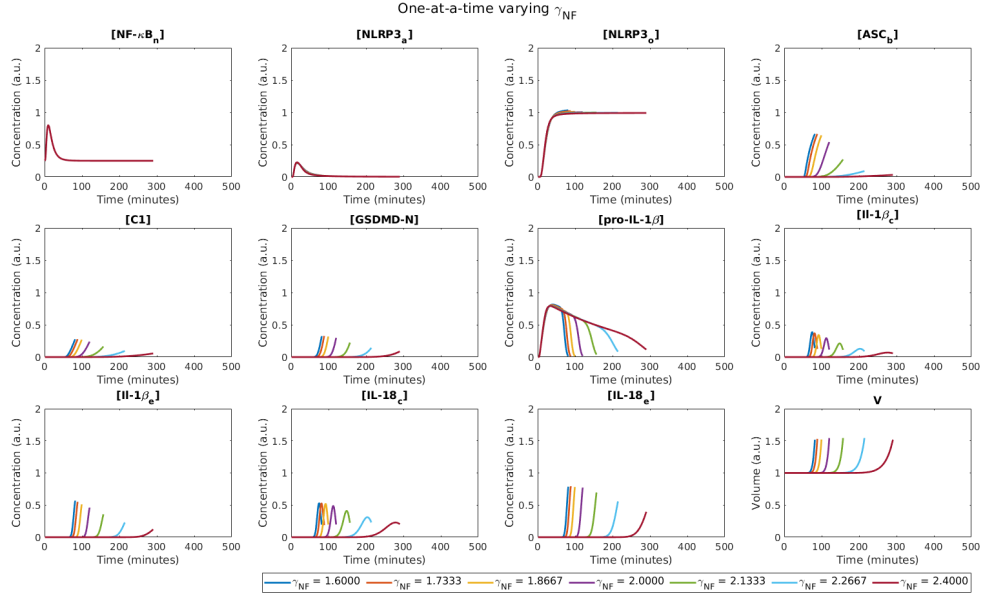

Figure S2.K: Numerical simulations results of the ODE model, while testing a range of values of the parameter  $\gamma_{NF}$  and fixing all other parameter values. We display the concentration of each model component in arbitrary units (a.u.) over time, as well as cell volume dynamics for each of the values tested. Note that the time progression stops once the critical volume  $V_c = 1.5$  is reached and the ultimate cell membrane rupture occurs.

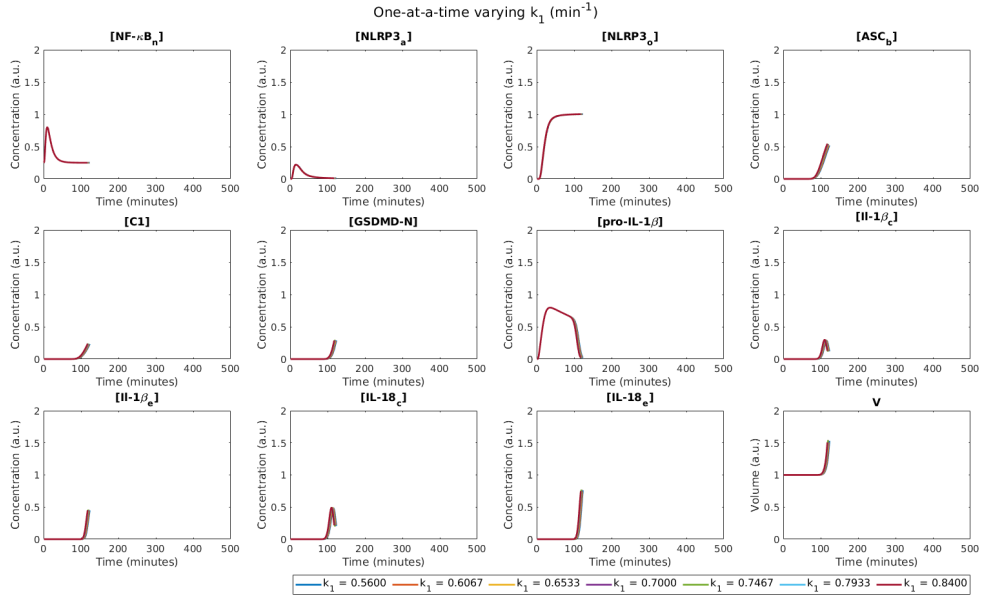

Figure S2.L: Numerical simulations results of the ODE model, while testing a range of values of the parameter  $k_1$  and fixing all other parameter values. We display the concentration of each model component in arbitrary units (a.u.) over time, as well as cell volume dynamics for each of the values tested. Note that the time progression stops once the critical volume  $V_c = 1.5$  is reached and the ultimate cell membrane rupture occurs.

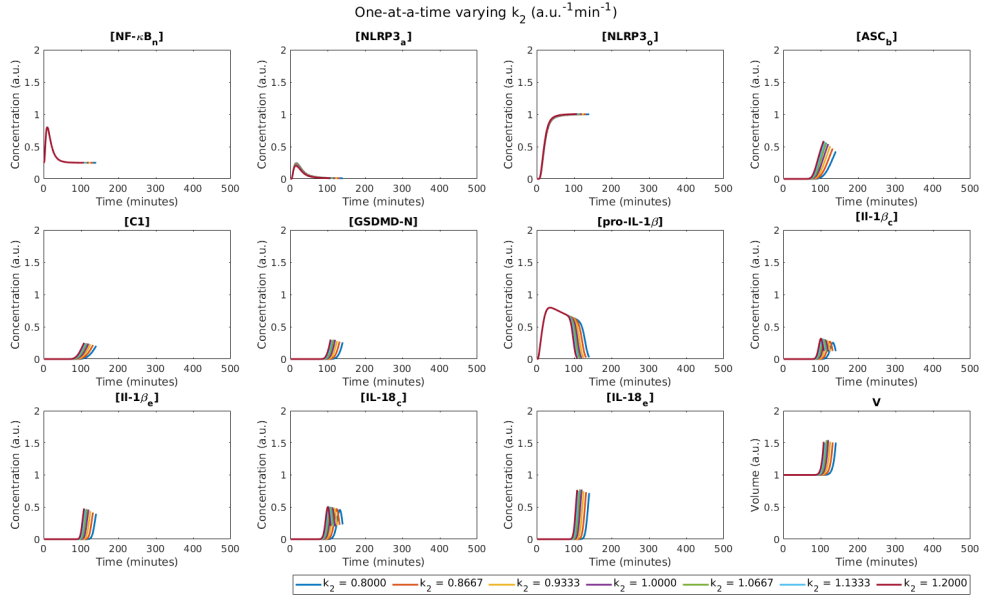

Figure S2.M: Numerical simulations results of the ODE model, while testing a range of values of the parameter  $k_2$  and fixing all other parameter values. We display the concentration of each model component in arbitrary units (a.u.) over time, as well as cell volume dynamics for each of the values tested. Note that the time progression stops once the critical volume  $V_c = 1.5$  is reached and the ultimate cell membrane rupture occurs.

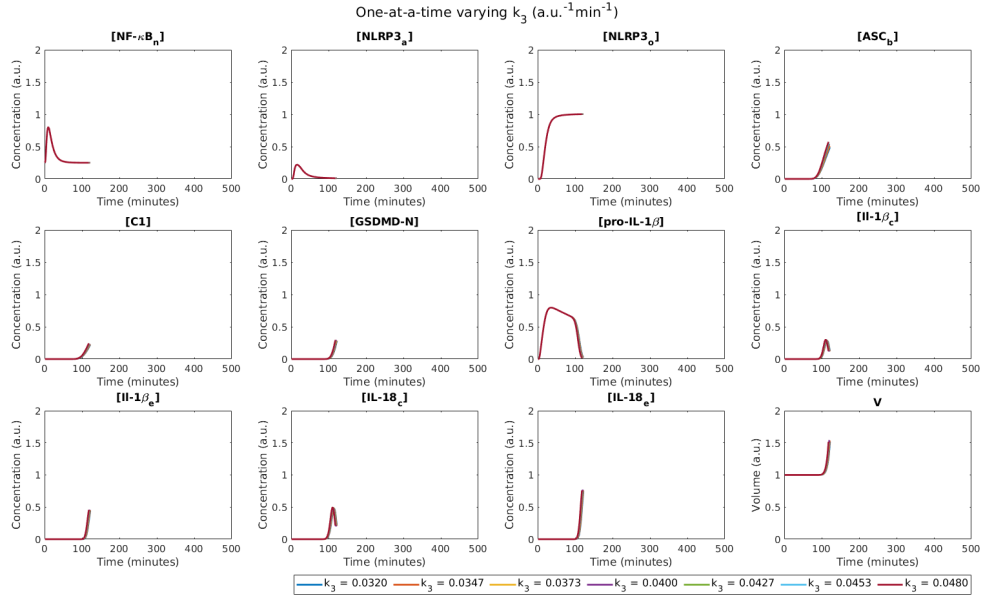

Figure S2.N: Numerical simulations results of the ODE model, while testing a range of values of the parameter  $k_3$  and fixing all other parameter values. We display the concentration of each model component in arbitrary units (a.u.) over time, as well as cell volume dynamics for each of the values tested. Note that the time progression stops once the critical volume  $V_c = 1.5$  is reached and the ultimate cell membrane rupture occurs.

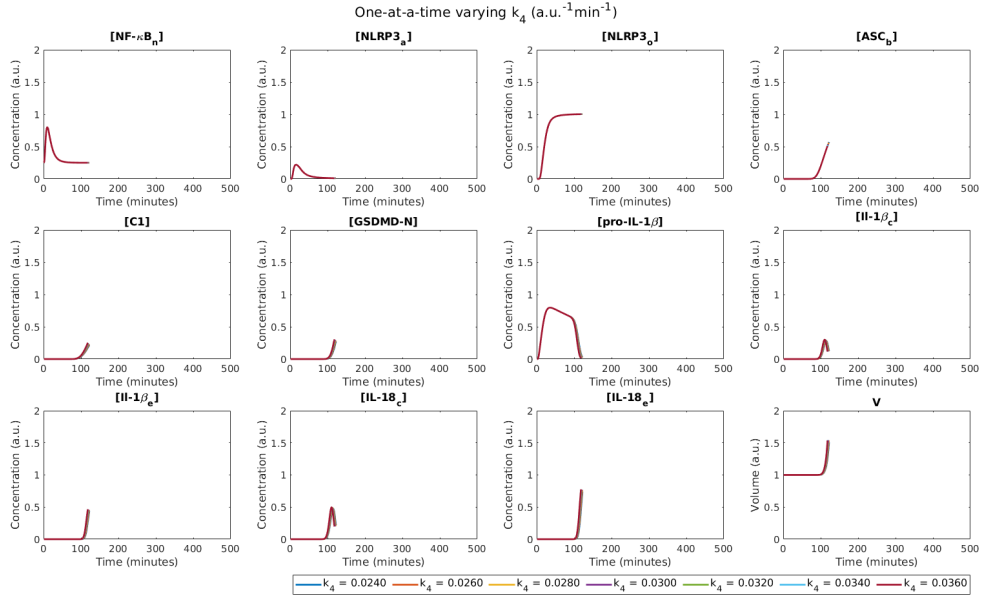

Figure S2.O: Numerical simulations results of the ODE model, while testing a range of values of the parameter  $k_4$  and fixing all other parameter values. We display the concentration of each model component in arbitrary units (a.u.) over time, as well as cell volume dynamics for each of the values tested. Note that the time progression stops once the critical volume  $V_c = 1.5$  is reached and the ultimate cell membrane rupture occurs.

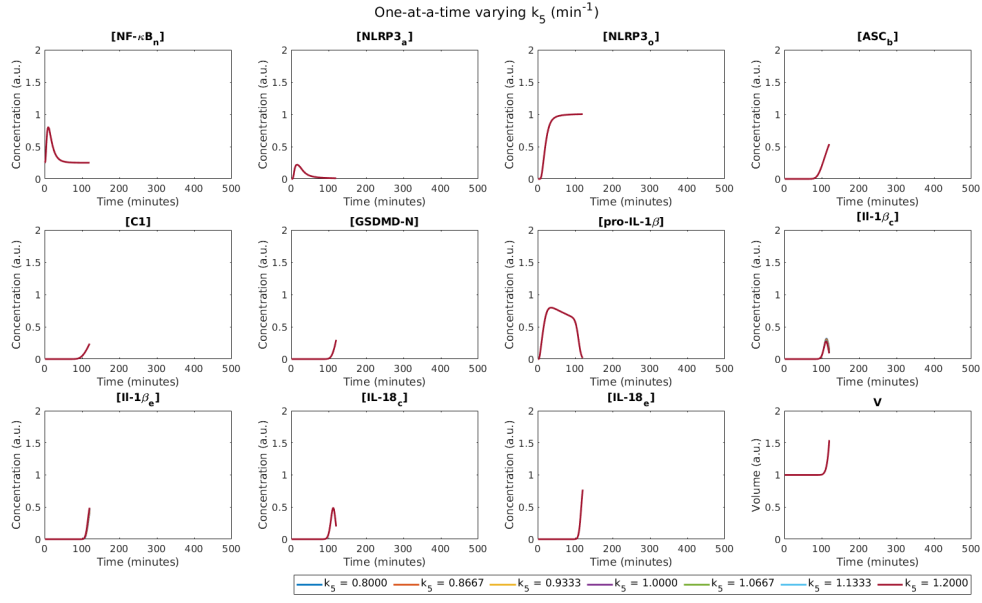

Figure S2.P: Numerical simulations results of the ODE model, while testing a range of values of the parameter  $k_5$  and fixing all other parameter values. We display the concentration of each model component in arbitrary units (a.u.) over time, as well as cell volume dynamics for each of the values tested. Note that the time progression stops once the critical volume  $V_c = 1.5$  is reached and the ultimate cell membrane rupture occurs.



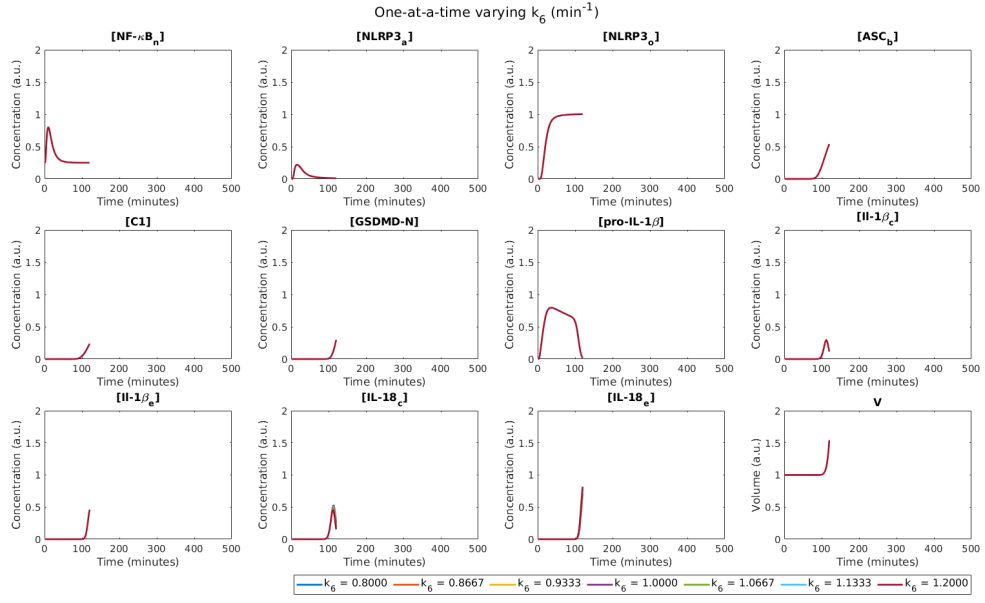

Figure S2.Q: Numerical simulations results of the ODE model, while testing a range of values of the parameter  $k_6$  and fixing all other parameter values. We display the concentration of each model component in arbitrary units (a.u.) over time, as well as cell volume dynamics for each of the values tested. Note that the time progression stops once the critical volume  $V_c = 1.5$  is reached and the ultimate cell membrane rupture occurs.

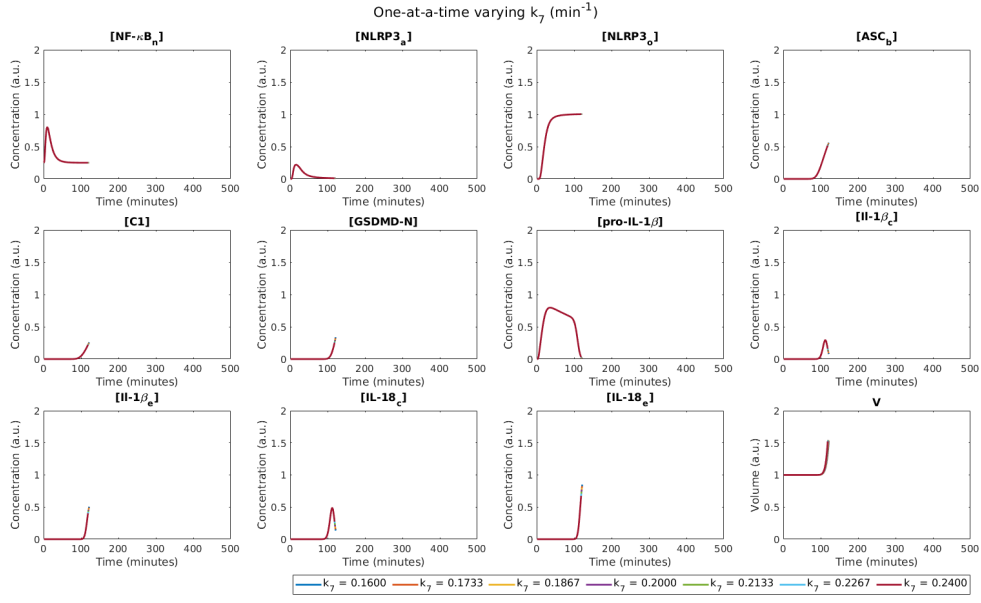

Figure S2.R: Numerical simulations results of the ODE model, while testing a range of values of the parameter  $k_7$  and fixing all other parameter values. We display the concentration of each model component in arbitrary units (a.u.) over time, as well as cell volume dynamics for each of the values tested. Note that the time progression stops once the critical volume  $V_c = 1.5$  is reached and the ultimate cell membrane rupture occurs.

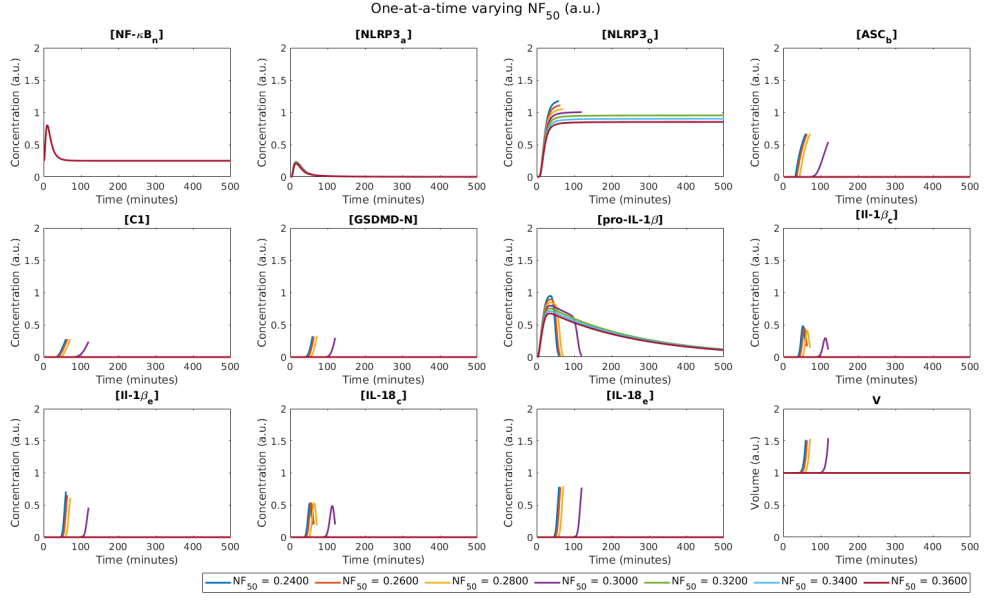

Figure S2.S: Numerical simulations results of the ODE model, while testing a range of values of the parameter  $NF_{50}$  and fixing all other parameter values. We display the concentration of each model component in arbitrary units (a.u.) over time, as well as cell volume dynamics for each of the values tested. Note that the time progression stops once the critical volume  $V_c = 1.5$  is reached and the ultimate cell membrane rupture occurs.

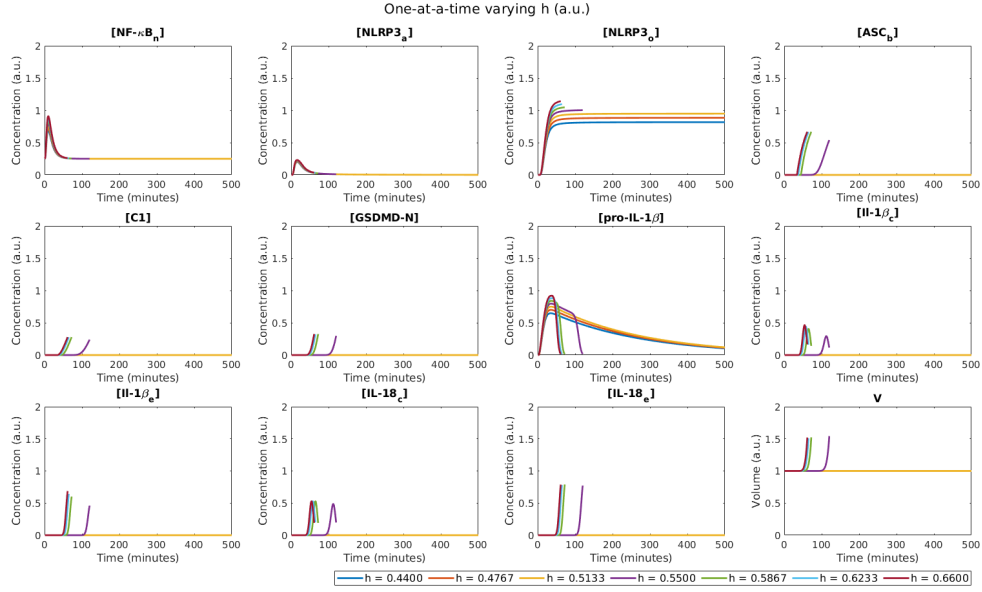

Figure S2.T: Numerical simulations results of the ODE model, while testing a range of values of the parameter  $h$  and fixing all other parameter values. We display the concentration of each model component in arbitrary units (a.u.) over time, as well as cell volume dynamics for each of the values tested. Note that the time progression stops once the critical volume  $V_c = 1.5$  is reached and the ultimate cell membrane rupture occurs.

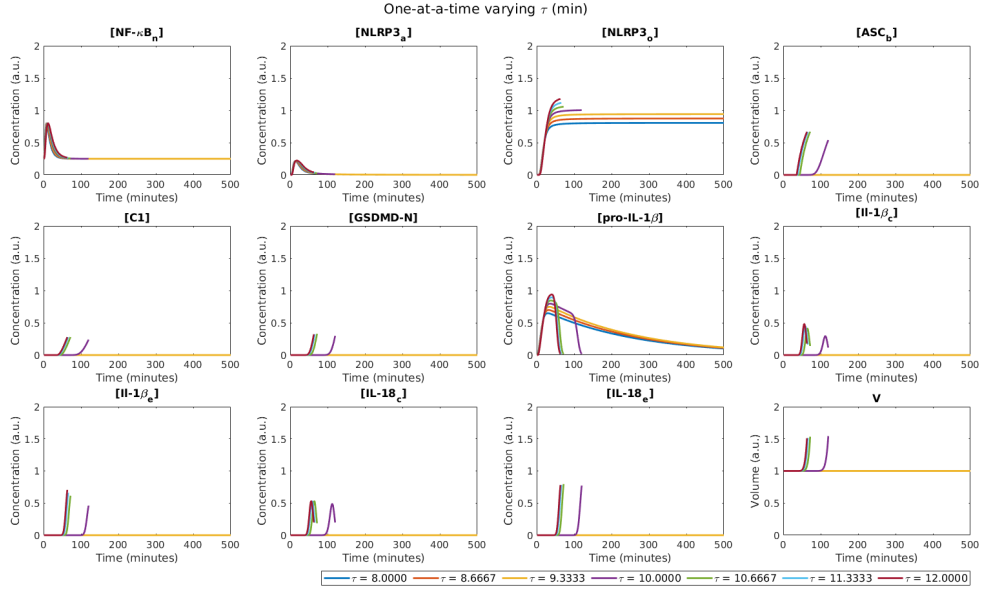

Figure S2.U: Numerical simulations results of the ODE model, while testing a range of values of the parameter  $\tau$  and fixing all other parameter values. We display the concentration of each model component in arbitrary units (a.u.) over time, as well as cell volume dynamics for each of the values tested. Note that the time progression stops once the critical volume  $V_c = 1.5$  is reached and the ultimate cell membrane rupture occurs.

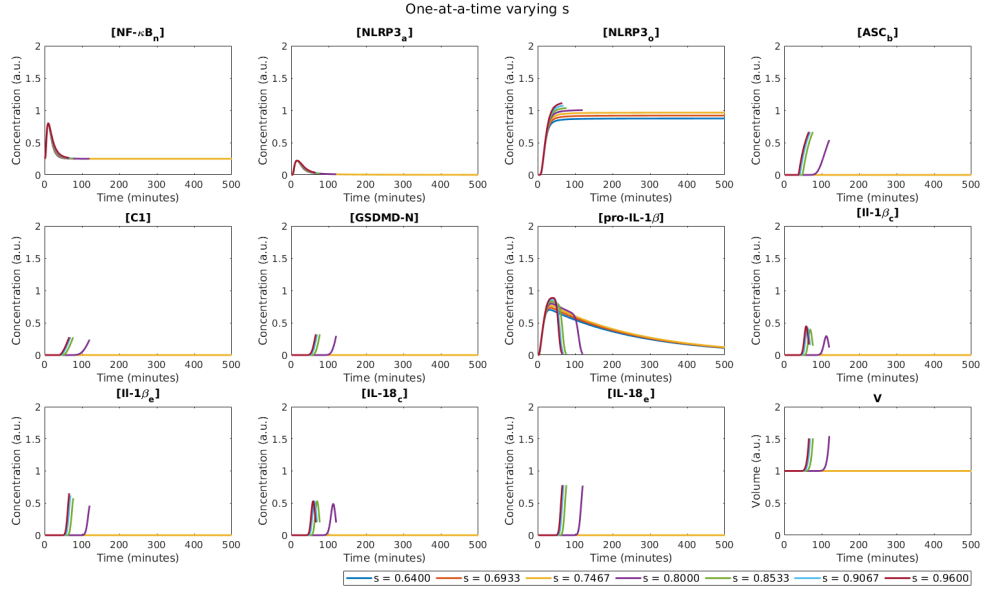

Figure S2.V: Numerical simulations results of the ODE model, while testing a range of values of the parameter  $s$  and fixing all other parameter values. We display the concentration of each model component in arbitrary units (a.u.) over time, as well as cell volume dynamics for each of the values tested. Note that the time progression stops once the critical volume  $V_c = 1.5$  is reached and the ultimate cell membrane rupture occurs.

## S3 Results from the global sensitivity analysis

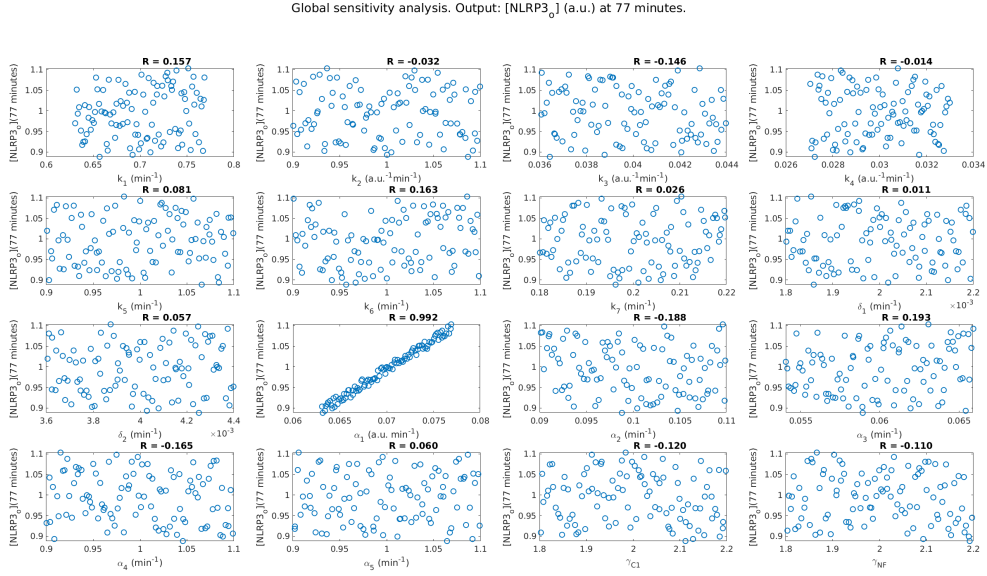

Figure S3.A: Global sensitivity analysis is performed using Latin hypercube sampling and analysis. The output, *i.e.*, the NLRP3<sub>o</sub> concentration (in arbitrary units of concentration) at 77 minutes, is plotted over three input parameters. Each input parameter range spans  $\pm 10\%$  of the estimated parameter value. The Pearson correlation coefficient (R), measuring the linear association between each input-output pair, is provided at the top right corner of each corresponding subplot.

## S4 Results from the derivative-based sensitivity analysis

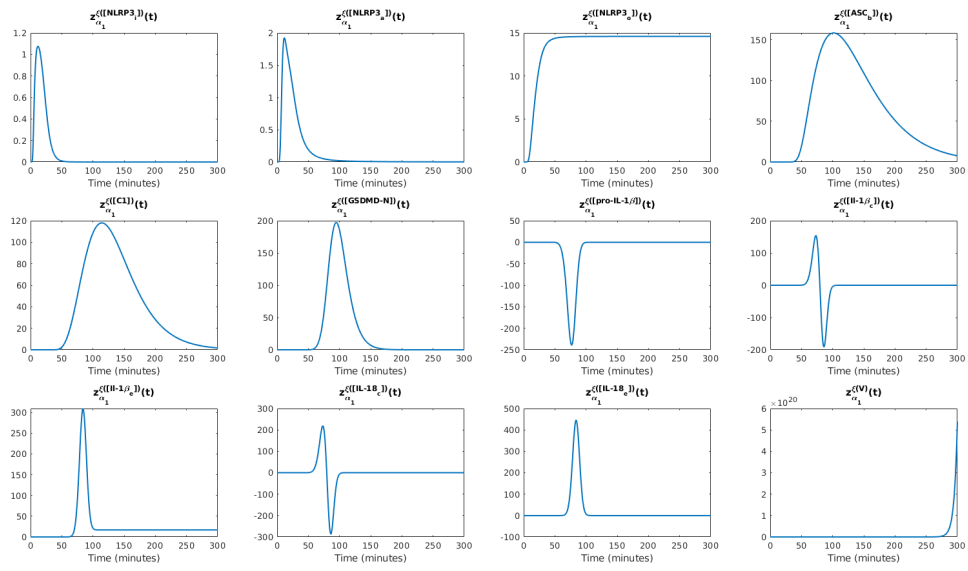

Figure S4.A: A derivative-based sensitivity analysis. Here  $z_j^i$  denotes the sensitivity of the output concentration computed in equation  $i$ , with respect to the input parameter  $\theta_j$ , where  $\xi(\text{compound concentration})$  maps each compound to its governing equation index  $i$ .

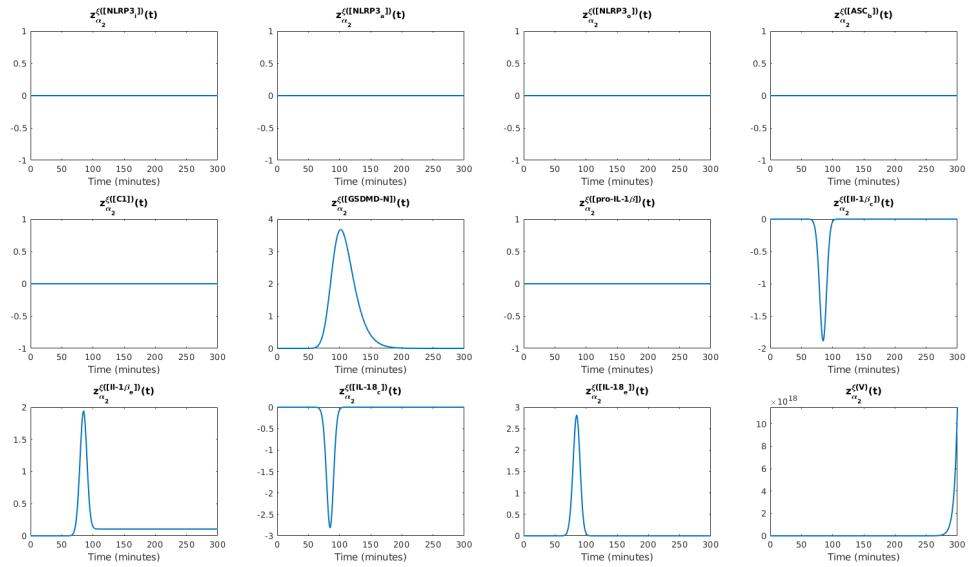

Figure S4.B: A derivative-based sensitivity analysis. Here  $z_j^i$  denotes the sensitivity of the output concentration computed in equation  $i$ , with respect to the input parameter  $\theta_j$ , where  $\xi(\text{compound concentration})$  maps each compound to its governing equation index  $i$ .



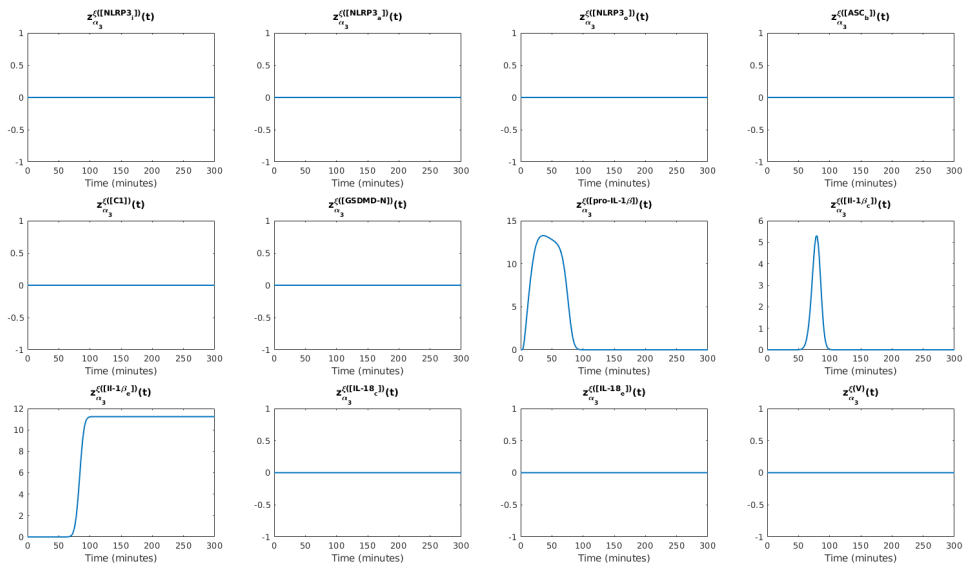

Figure S4.C: A derivative-based sensitivity analysis. Here  $z_j^i$  denotes the sensitivity of the output concentration computed in equation  $i$ , with respect to the input parameter  $\theta_j$ , where  $\xi(\text{compound concentration})$  maps each compound to its governing equation index  $i$ .

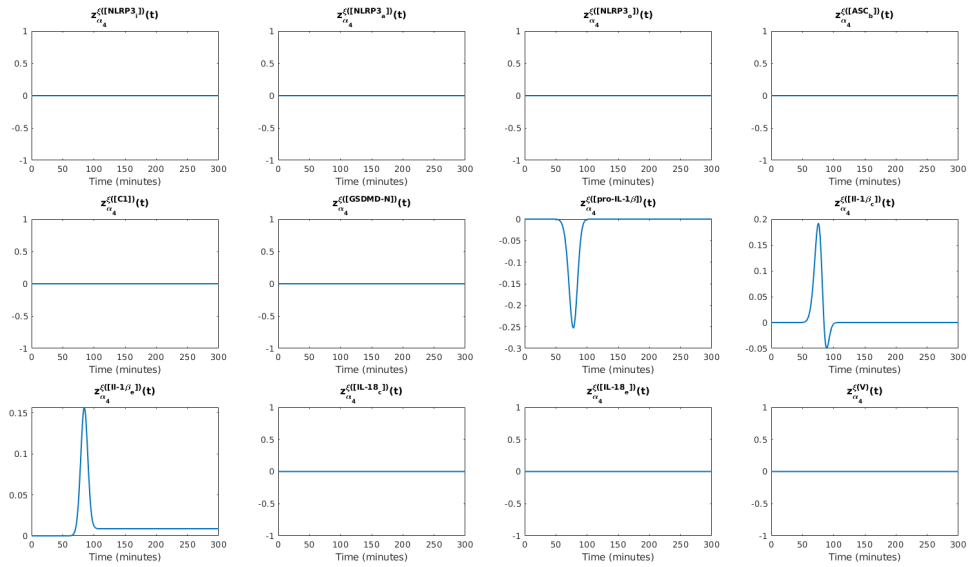

Figure S4.D: A derivative-based sensitivity analysis. Here  $z_j^i$  denotes the sensitivity of the output concentration computed in equation  $i$ , with respect to the input parameter  $\theta_j$ , where  $\xi(\text{compound concentration})$  maps each compound to its governing equation index  $i$ .

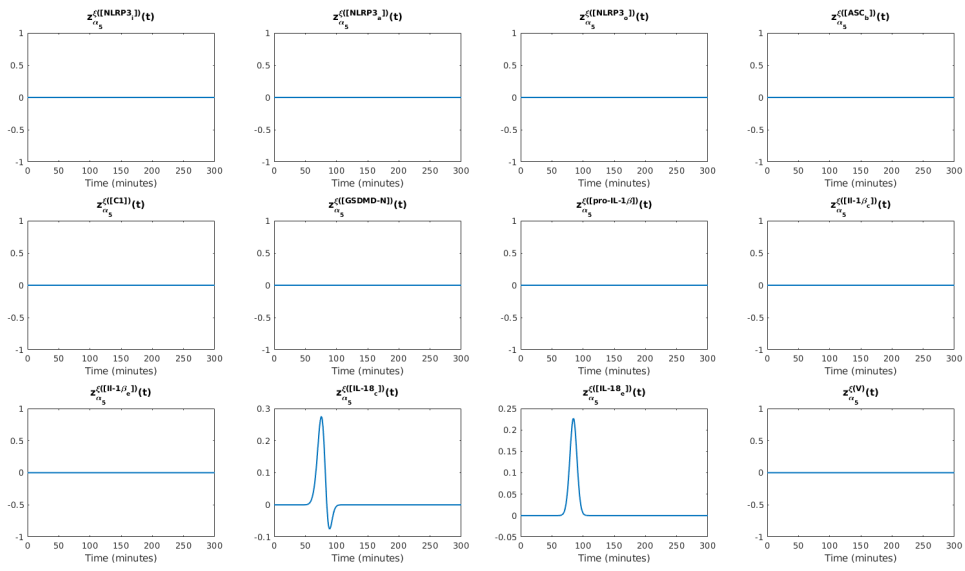

Figure S4.E: A derivative-based sensitivity analysis. Here  $z_j^i$  denotes the sensitivity of the output concentration computed in equation  $i$ , with respect to the input parameter  $\theta_j$ , where  $\xi(\text{compound concentration})$  maps each compound to its governing equation index  $i$ .

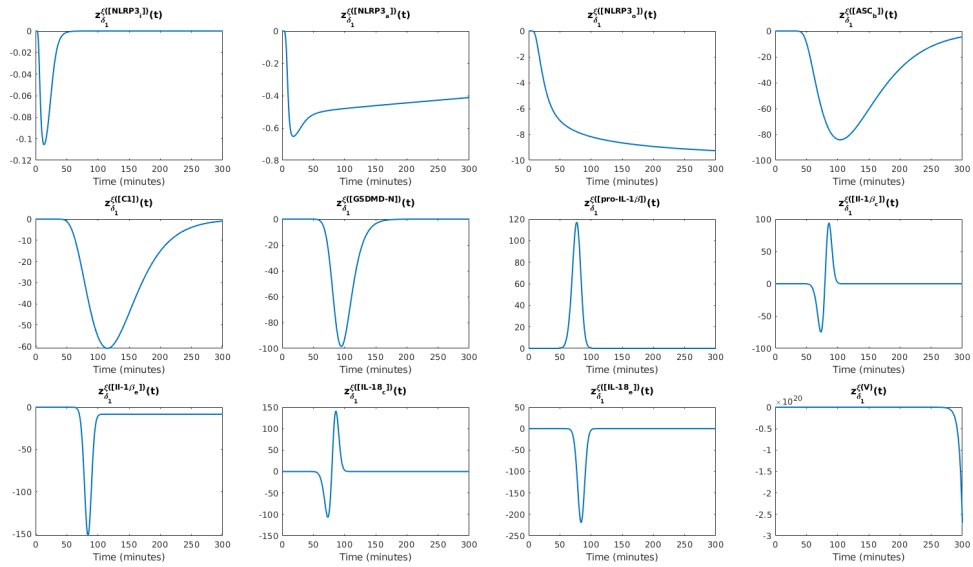

Figure S4.F: A derivative-based sensitivity analysis. Here  $z_j^i$  denotes the sensitivity of the output concentration computed in equation  $i$ , with respect to the input parameter  $\theta_j$ , where  $\xi(\text{compound concentration})$  maps each compound to its governing equation index  $i$ .

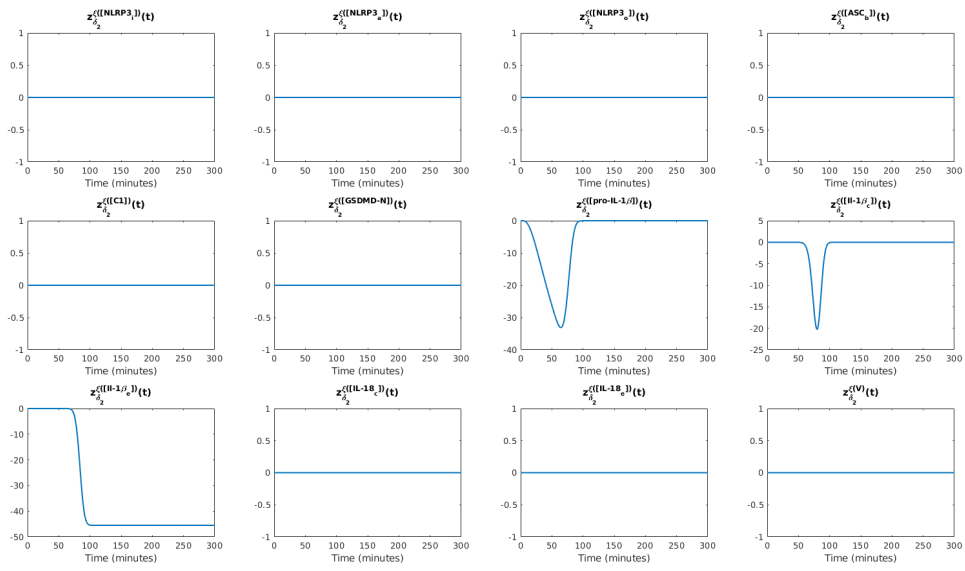

Figure S4.G: A derivative-based sensitivity analysis. Here  $z_j^i$  denotes the sensitivity of the output concentration computed in equation  $i$ , with respect to the input parameter  $\theta_j$ , where  $\xi(\text{compound concentration})$  maps each compound to its governing equation index  $i$ .

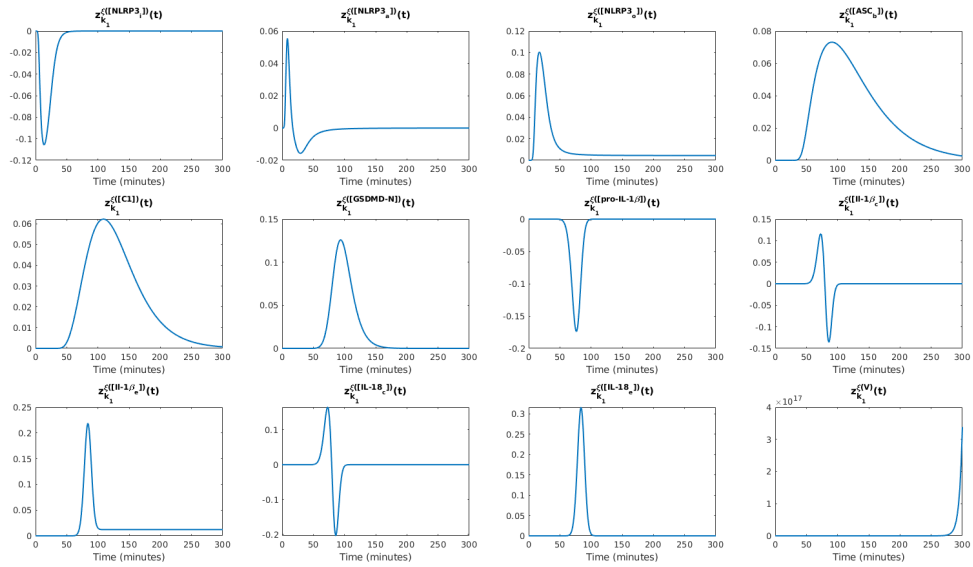

Figure S4.H: A derivative-based sensitivity analysis. Here  $z_j^i$  denotes the sensitivity of the output concentration computed in equation  $i$ , with respect to the input parameter  $\theta_j$ , where  $\xi(\text{compound concentration})$  maps each compound to its governing equation index  $i$ .

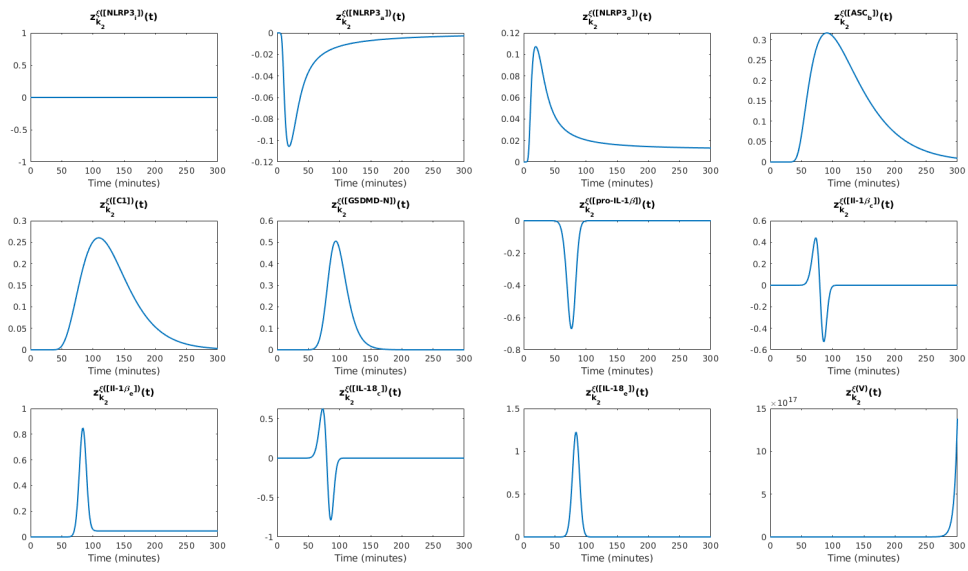

Figure S4.I: A derivative-based sensitivity analysis. Here  $z_j^i$  denotes the sensitivity of the output concentration computed in equation  $i$ , with respect to the input parameter  $\theta_j$ , where  $\xi$ (compound concentration) maps each compound to its governing equation index  $i$ .

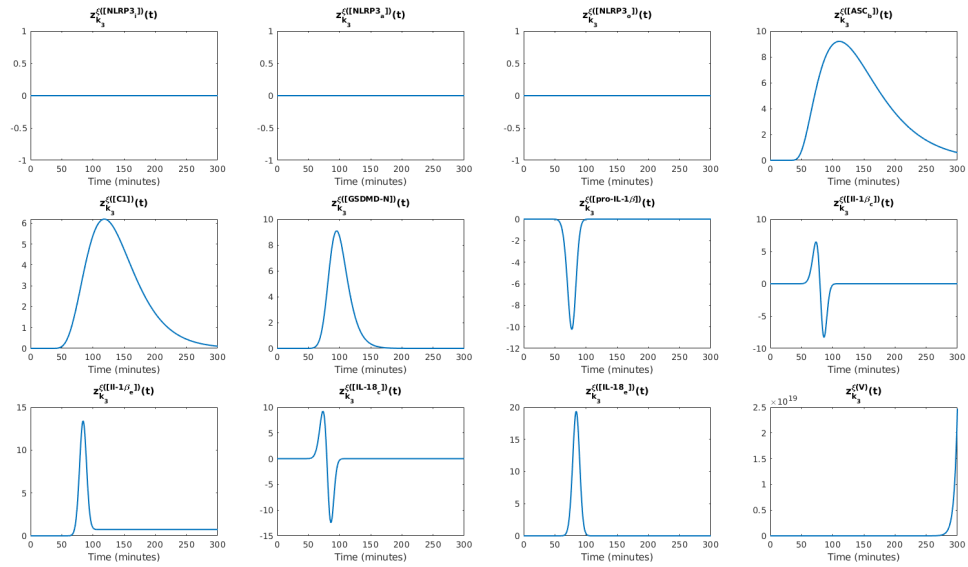

Figure S4.J: A derivative-based sensitivity analysis. Here  $z_j^i$  denotes the sensitivity of the output concentration computed in equation  $i$ , with respect to the input parameter  $\theta_j$ , where  $\xi$ (compound concentration) maps each compound to its governing equation index  $i$ .

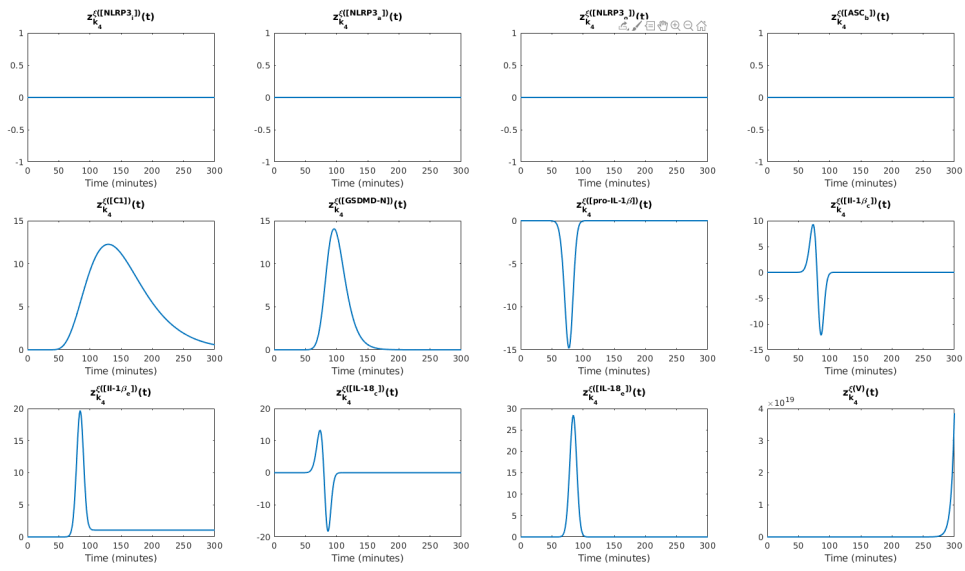

Figure S4.K: A derivative-based sensitivity analysis. Here  $z_j^i$  denotes the sensitivity of the output concentration computed in equation  $i$ , with respect to the input parameter  $\theta_j$ , where  $\xi(\text{compound concentration})$  maps each compound to its governing equation index  $i$ .

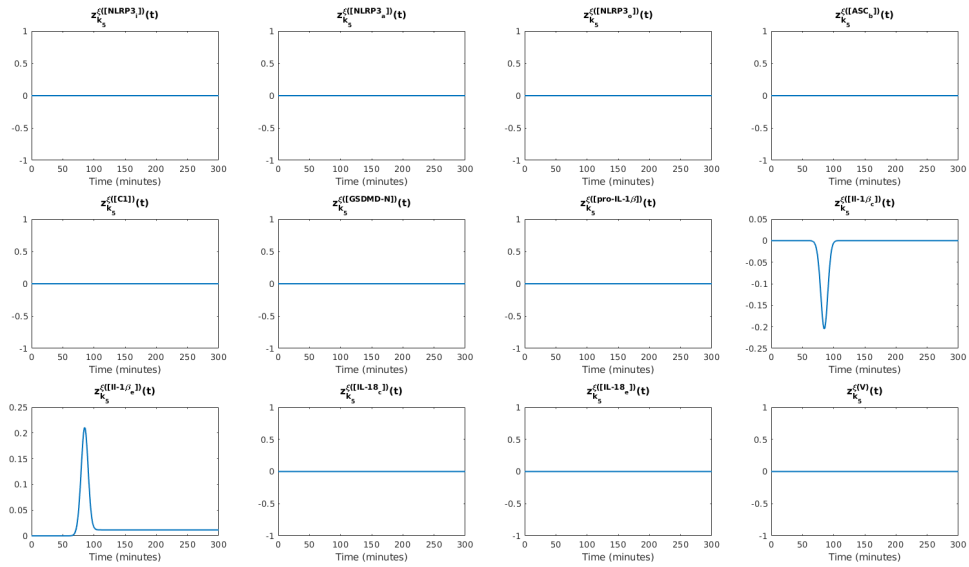

Figure S4.L: A derivative-based sensitivity analysis. Here  $z_j^i$  denotes the sensitivity of the output concentration computed in equation  $i$ , with respect to the input parameter  $\theta_j$ , where  $\xi(\text{compound concentration})$  maps each compound to its governing equation index  $i$ .

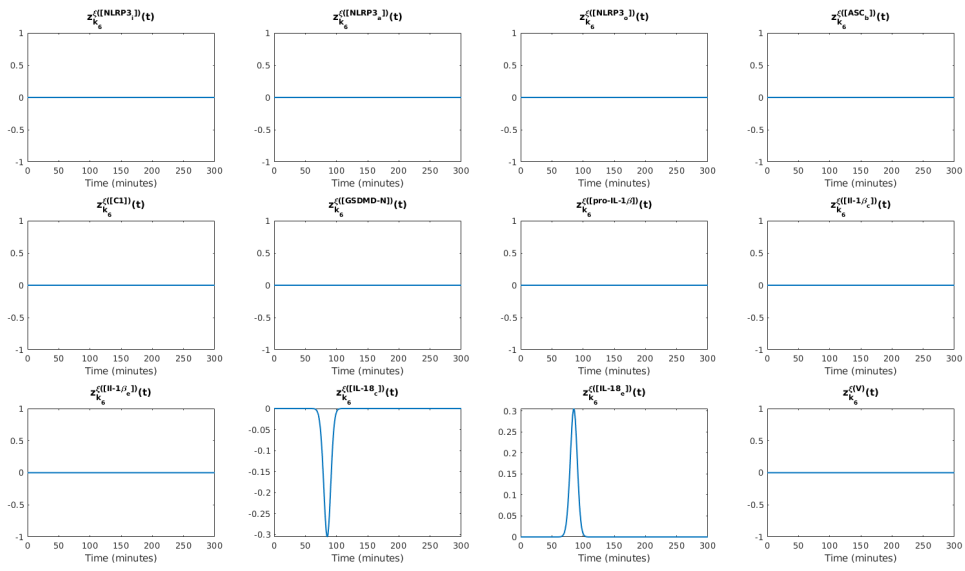

Figure S4.M: A derivative-based sensitivity analysis. Here  $z_j^i$  denotes the sensitivity of the output concentration computed in equation  $i$ , with respect to the input parameter  $\theta_j$ , where  $\xi(\text{compound concentration})$  maps each compound to its governing equation index  $i$ .

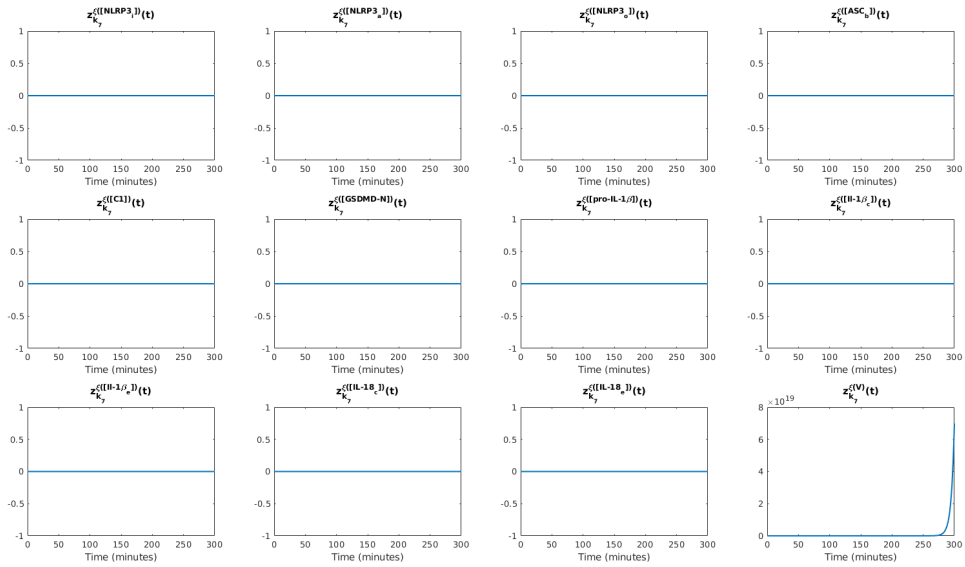

Figure S4.N: A derivative-based sensitivity analysis. Here  $z_j^i$  denotes the sensitivity of the output concentration computed in equation  $i$ , with respect to the input parameter  $\theta_j$ , where  $\xi(\text{compound concentration})$  maps each compound to its governing equation index  $i$ .

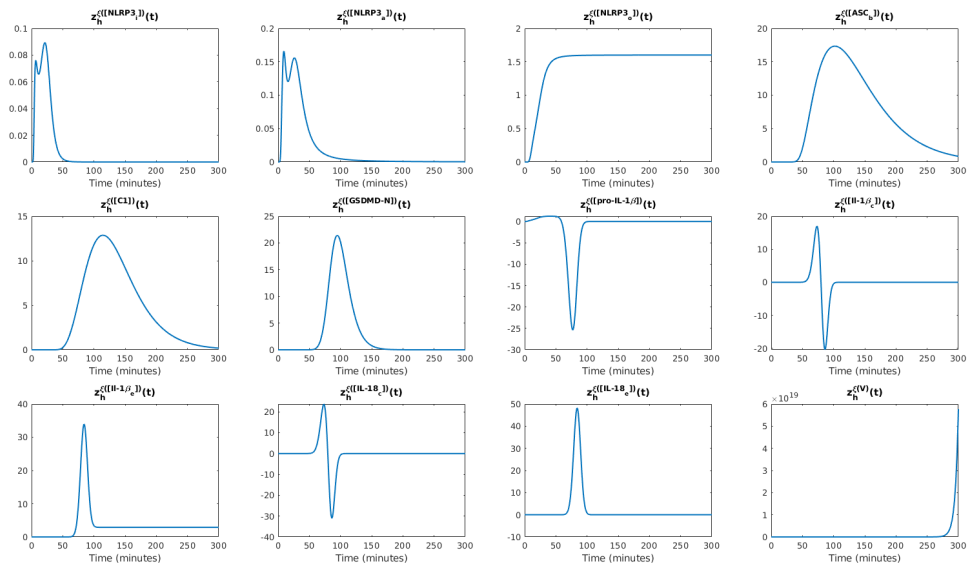

Figure S4.O: A derivative-based sensitivity analysis. Here  $z_j^i$  denotes the sensitivity of the output concentration computed in equation  $i$ , with respect to the input parameter  $\theta_j$ , where  $\xi(\text{compound concentration})$  maps each compound to its governing equation index  $i$ .

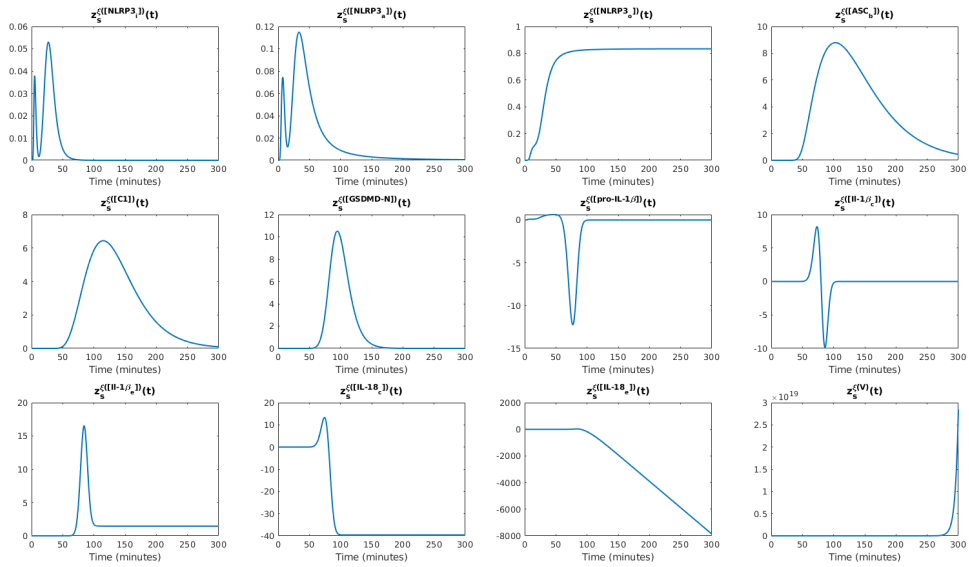

Figure S4.P: A derivative-based sensitivity analysis. Here  $z_j^i$  denotes the sensitivity of the output concentration computed in equation  $i$ , with respect to the input parameter  $\theta_j$ , where  $\xi(\text{compound concentration})$  maps each compound to its governing equation index  $i$ .

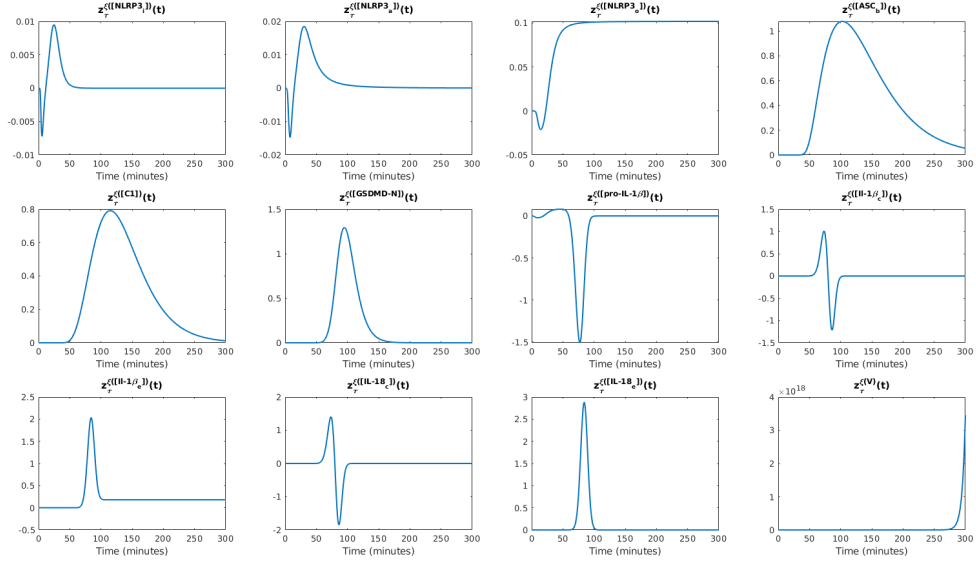

Figure S4.Q: A derivative-based sensitivity analysis. Here  $z_j^i$  denotes the sensitivity of the output concentration computed in equation  $i$ , with respect to the input parameter  $\theta_j$ , where  $\xi(\text{compound concentration})$  maps each compound to its governing equation index  $i$ .

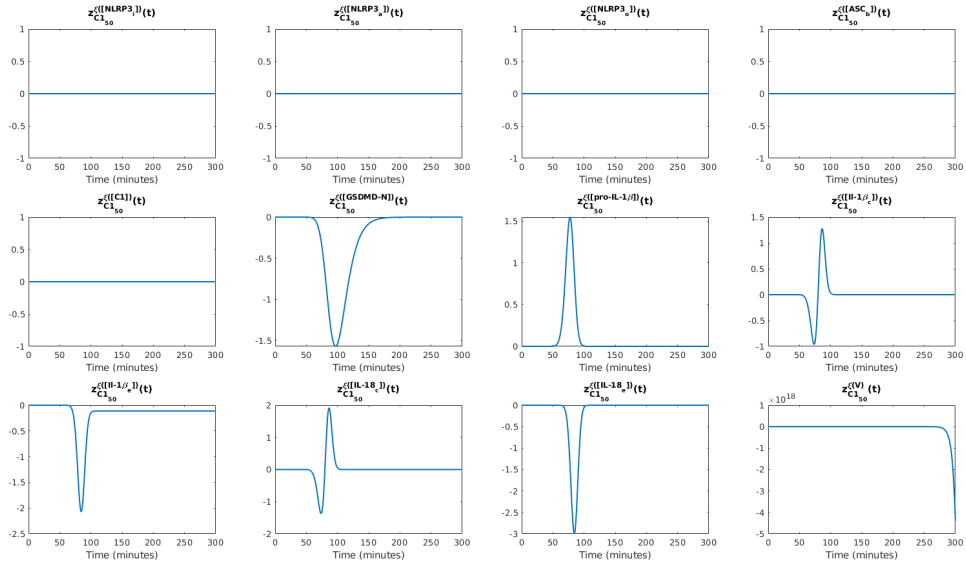

Figure S4.R: A derivative-based sensitivity analysis. Here  $z_j^i$  denotes the sensitivity of the output concentration computed in equation  $i$ , with respect to the input parameter  $\theta_j$ , where  $\xi(\text{compound concentration})$  maps each compound to its governing equation index  $i$ .



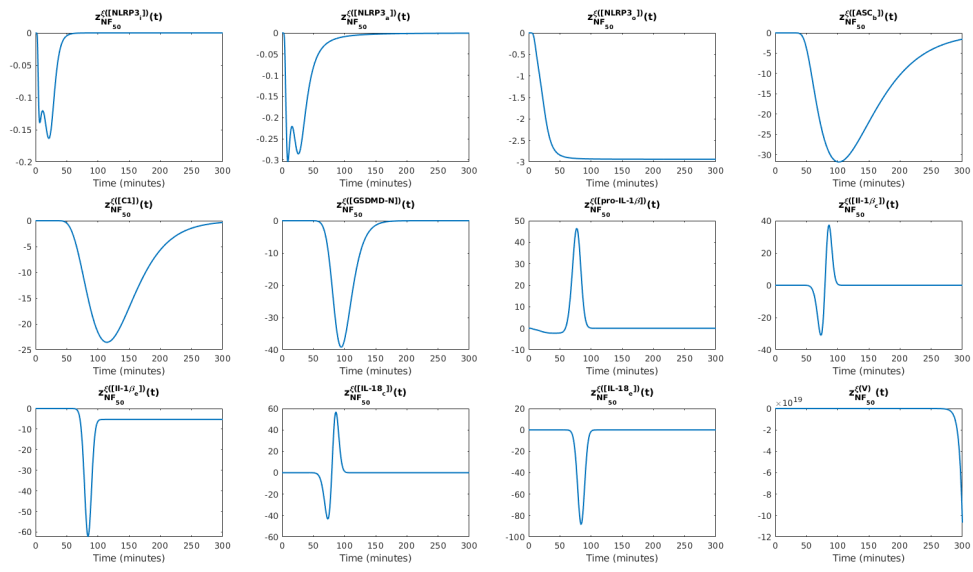

Figure S4.S: A derivative-based sensitivity analysis. Here  $z_j^i$  denotes the sensitivity of the output concentration computed in equation  $i$ , with respect to the input parameter  $\theta_j$ , where  $\xi(\text{compound concentration})$  maps each compound to its governing equation index  $i$ .
